# Supplementary material for: The magnetic exciton of EuS revealed by resonant inelastic x-ray scattering
Source: arXiv:2310.18096 ancillary file (2023-10-27)
Supplement: Supplementary file 1 [file supplemental_material.pdf]

# Supplemental material
# for
# The magnetic exciton of EuS revealed by resonant inelastic x-ray scattering

Lucia Amidani*
*The Rossendorf Beamline (ROBL) at the ESRF,*
*71 Avenue des Martyrs, Grenoble 38043, France and*
*Institute of Resource Ecology, Helmholtz-Zentrum Dresden-Rossendorf (HZDR),*
*Bautzner Landstraße 400, 01328 Dresden, Germany*

Jonas J. Joos
*Lumilab, Department of Solid State Sciences, Ghent University, Krijgslaan 281-S1, B-9000 Gent, Belgium*

Pieter Glatzel
*ESRF – The European Synchrotron, 71 Avenue des Martyrs, 38000 Grenoble, France*

Jindřich Kolorenč†
*Institute of Physics (FZU), Czech Academy of Sciences, Na Slovance 2, 182 00 Prague, Czech Republic*
(Dated: October 27, 2023)

Here we provide details on (i) sample synthesis, (ii) RIXS instrumentation and measurements, (iii) LDA+DMFT calculations, (iv) open-core LDA calculations, (v) modeling the localized excitons in supercells using the open-core approximation, (vi) estimation of the intensity of the 4f → 2p quadrupolar emission, and on (vii) indirect RIXS processes.

## NOTATION

Numbers of sections, figures, tables, equations and references in this supplemental material are prefixed with letter "S". Numbers without prefix refer to the figures and equations from the main article.

## S.I. SAMPLE PREPARATION

The EuS powder was synthesized by sulfurizing high-purity $Eu_2O_3$ (Alfa Aesar, 99.99%) in a stream of $H_2S$ at 900 °C. The purity of the obtained powders was verified with x-ray diffraction (XRD).

The EuS powder (10 mg) was mixed with boron nitride and pressed into 13 mm pellets for RIXS measurements. We checked for sample damage by collecting consecutive fast HERFD-XANES at the Eu $L_3$ edge on different spots. The sample was stable under the beam.

## S.II. RIXS MEASUREMENTS

Valence-to-core resonant inelastic x-ray scattering (RIXS) at the Eu $L_3$ edge was measured on the ID26 beamline at the ESRF [S1]. The incident beam energy was selected and scanned with a fixed-exit Si(311) double-crystal monochromator. The scattered x-rays were analyzed with the ID26 hard x-ray emission spectrometer based on Rowland geometry equipped with a set of five Si(531) bent crystal analyzers. Photons with the scattering angle (measured between the incident beam and the outgoing photon) in the range from 72° to 107° were detected. The RIXS planes were obtained by collecting scans of the emission spectrometer around the energy of the incident beam at several incident energies in the region of the absorption edge. The energy-transfer axis of RIXS was aligned by fitting the elastic peak and by setting the maximum as the origin. The emission spectrometer was scanned across the energy of the incoming beam to acquire an energy-transfer range between −2 eV and 16 eV.

## S.III. LDA+DMFT

To model the electronic structure of the sulfide, we employ the LDA+DMFT method in the implementation described in [S3, S4]. First, the non-magnetic (spin-restricted) band structure calculated in the local density approximation (LDA) is represented by a tight-binding model in the basis of the maximally localized Wannier functions, and then a momentum-independent self-energy is inserted into the europium 4f shells to improve the description of the localized 4f electrons. This self-energy is obtained by solving an auxiliary impurity model representing one interacting 4f shell embedded in an appropriate non-interacting crystalline environment (often referred to as the bath). This solution is found using the Lanczos method.

The starting LDA band structure is calculated using Wien2k software [S5], which implements the linearized augmented plane-wave method (LAPW) and its extensions. The core states (Eu up to 4d, S up to 2p) are evaluated in the corresponding muffin-tin spheres by nu-

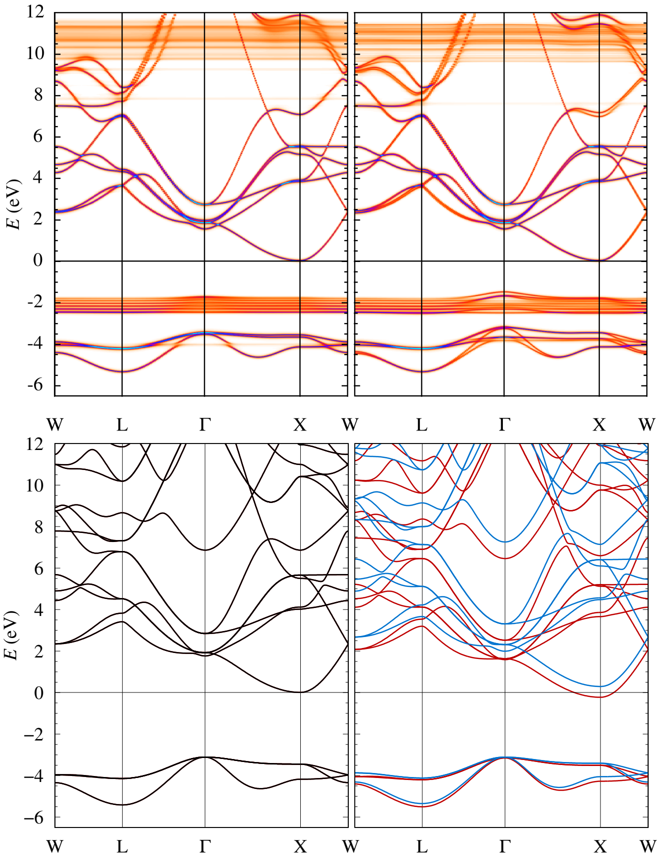


FIG. S1. Band structure (Bloch spectral function) of EuS: LDA+DMFT in the top row (paramagnetic solution on the left, ferromagnetic solution with moments pointing along [001] on the right), and open-core LDA in the bottom row (non-magnetic solution on the left, ferromagnetic solution on the right with majority and minority spins distinguished by color). The band structures are aligned such that the bottom of the 5d bands is at zero energy. In the spin-polarized states, we align the average of the majority-spin and minority-spin bands.

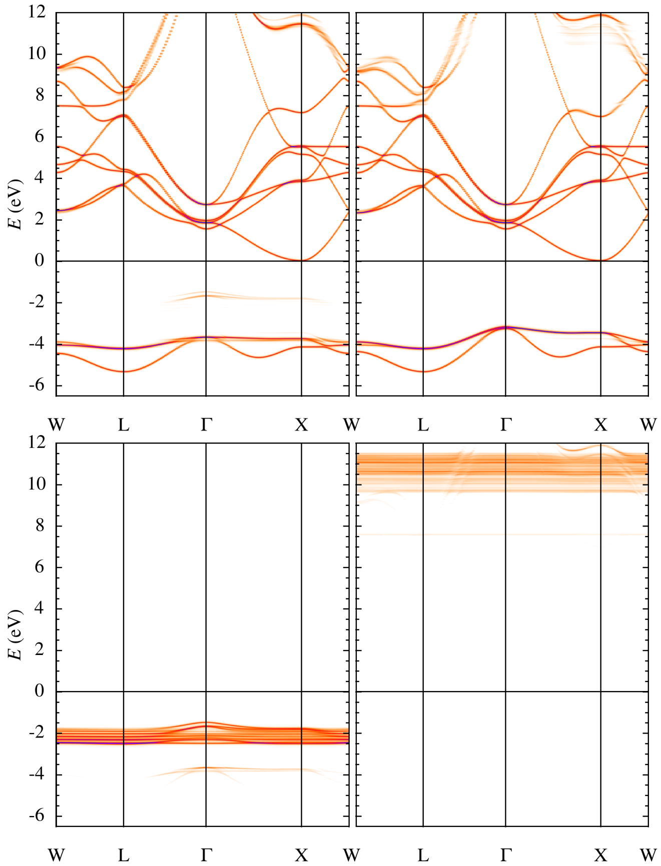


FIG. S2. Band structure (Bloch spectral function) of EuS in the ferromagnetic LDA+DMFT solution. Majority-spin states on the left, minority-spin states on the right. We plot separately non-4f states (top) and 4f states (bottom). Note the hybridization between Eu 4f and S 3p states visible in the majority-spin channel, which is consistent with the recent ARPES measurements [S2].

merically exact integration of the Kohn–Sham–Dirac equations. All higher-lying states are considered as the valence states, for which the method combines a scalar-relativistic description with spin-orbit coupling added in a second variational step. The radii of muffin-tin spheres for individual atoms are $R_{\mathrm{MT}}(\mathrm{Eu}) = 2.8\ a_{\mathrm{B}}$ and $R_{\mathrm{MT}}(\mathrm{S}) = 2.5\ a_{\mathrm{B}}$, the plane-wave cutoff $K_{\max}$ is set by $R_{\mathrm{MT}}(\mathrm{S}) \times K_{\max} = 8$, and the Brillouin zone is sampled with a $15 \times 15 \times 15$ mesh in the self-consistency cycle (a denser mesh is used for plotting densities of states). In all calculations, we use the experimental lattice constant of EuS, $a_0 = 5.968$ Å [S6], and we do not perform any geometry optimization.

The tight-binding model is constructed with the aid of Wannier90 code [S7, S8] and contains europium 4f, 5d, 6s, 6p and sulfur 3p states. This basis allows for an accurate representation of the original LDA band structure up to 7 eV above the Fermi level, higher-lying bands are represented only approximately or they are missing. The quality of the representation can be inferred from Fig. S1.

Since the gap between the S 3p and Eu 5d bands is underestimated in LDA, we shift the S 3p bands to higher binding energies by reducing the S 3p orbital energies in the tight-binding model by 1.5 eV. The gap between the S 3p and Eu 5d states affects the covalent mixing of these states, which in turn influences the intensity of the dipole-allowed RIXS signal, since the emission happens from Eu 5d states mixed into the nominally S 3p bands. There are more sophisticated methods to correct the LDA band-gap problem that were applied to Eu chalcogenides in the past, such as the *GW* method [S9], orbital-dependent hybrid exchange-correlation functionals [S10] or advanced semi-local exchange-correlation functionals [S2]. For our purposes, the simple shift of the S 3p orbital energies should be sufficient since all these methods result in a very similar electronic structure anyway.

The Coulomb interaction in the 4f shell is considered in the spherically symmetric form as in an ion, characterized by four Slater parameters $F_0 = 7.0$ eV, $F_2 = 12.1$ eV,

$F_4 = 7.7$ eV, and $F_6 = 5.5$ eV, which correspond to Coulomb $U = F_0 = 7.0$ eV and Hund

$$J = \frac{2\ell+1}{2\ell} \sum_{k=1}^{\ell} F_{2k} \begin{pmatrix} \ell & 2k & \ell \\ 0 & 0 & 0 \end{pmatrix}^2 = 1.0 \text{ eV}. \qquad \text{(S1)}$$

The first parameter is chosen empirically, we use the same value as previously employed in [S11]. The other three parameters ($F_2$, $F_4$, $F_6$) correspond to the atomic Hartree–Fock values calculated for the $Eu^{2+}$ ion ($4f^7$ configuration) and then reduced to 80% to simulate screening and multiconfigurational effects [S12, S13].

The double-counting correction is chosen empirically to place the occupied Eu 4f states such that the gap between them and the empty 5d bands ($\approx 1.6$ eV) is compatible with the optical absorption measurements [S6]. The above-mentioned shift of the S 3p bands then makes the final electronic structure compatible also with the valence-band photoemission [S14] that suggests $\approx 2$ eV separation between maxima of the features corresponding to the Eu 4f and S 3p bands. Reference S14 reports the photoemission only for EuO and EuSe where the Eu 4f and O 2p (or Se 4p) distance is 2.8 eV and 1.6 eV, respectively. The EuS gap must be roughly in the middle of these two values.

In the auxiliary impurity model of our DMFT method, there are 14 bath orbitals below the Fermi level (nominally filled, representing the S 3p states) and 28 bath orbitals above the Fermi level (nominally empty, representing Eu 5d, 6s, and 6p states). We employ a Hilbert-space truncation to reduce the computational demands of the impurity solver, which amounts to limiting the number of deviations $M$ from the nominal occupations of the bath orbitals [S3, S4]. In the present calculations, we set $M = 2$ but the difference between $M = 1$ and $M = 2$ is negligible since the hybridization between Eu 4f states and the other states is very small.

We performed two types of calculations, one at a finite temperature (100 K introduced in the impurity solver), which converged to the paramagnetic state, and the other at zero temperature with a small symmetry-breaking field added in the initial iterations of the self-consistent loop, which converged to the ferromagnetic state. The final LDA+DMFT band structures for the paramagnetic and ferromagnetic phases are plotted in Fig. S1, the spin-resolved representation of the ferromagnetic state is shown in Fig. S2. Our calculations closely reproduce the behavior recently observed by high-resolution ARPES, namely the 4f states starting to show a dispersion near the $\Gamma$ point and the top of the S 3p band acquiring an exchange splitting after cooling to the ferromagnetic state, both effects being induced by hybridization between the Eu 4f and S 3p states [S2]. Figures S1 and S2 indicate that there is essentially no exchange splitting of the Eu 5d bands, which is a deficiency of our charge-non-selfconsistent LDA+DMFT implementation based on the spin-restricted LDA band structure as was discussed in detail elsewhere [S4].

## S.IV. OPEN-CORE APPROXIMATION

A conceptually simpler approximation designed for modeling localized 4f electrons in the DFT framework is the open-core method. It treats the 4f states as a part of the atomic core, which means they are assumed spherically symmetric, not contributing to the chemical bonding, and their filling is given a priori, as opposed to being determined self-consistently [S15–S17].

In the LAPW method, the core states are assumed to have their charge density confined within the muffin-tin sphere, a core charge leaking outside the sphere is a source of a bias. To reduce the leakage of the 4f charge, we increased the Eu muffin-tin radius to $R_{\mathrm{MT}}(\mathrm{Eu}) = 3.1\ a_{\mathrm{B}}$ in all open-core calculations, which results in 0.11, 0.18, 0.02, and 0.02 of 4f electron outside the Eu sphere for $4f^7$ spin-polarized, $4f^7$ spin-restricted, $4f^6$ spin-polarized, and $4f^6$ spin-restricted states.

The Kohn–Sham–Dirac core solver implemented in Wien2k code does not directly support spin-polarized potentials or unequal $\uparrow$ and $\downarrow$ electron densities. It assumes the single-electron levels to be $2j+1$ degenerate and labeled by the principal quantum number $\nu$ and Dirac quantum number $\kappa = \mp(j+1/2)$, where $j$ is the total angular momentum (we use $\kappa$ and $j$ interchangeably in the rest of the discussion). The core-electron density of one spin channel $\rho_\sigma$ in a spin-polarized state is then approximated by a half of the electron density of an auxiliary atomic core experiencing a radial potential $v = v_\sigma$ and having occupation numbers of the core levels $n_{\nu\kappa} = 2n_{\nu\kappa\sigma}$, where the numbers $n_{\nu\kappa\sigma}$ specify the approximate core state. This approximation was demonstrated to be very accurate in the standard DFT calculations, in which all core levels are fully occupied [S18]. The partially occupied open-core 4f level will be a source of some additional inaccuracies in the total energy, but we expect these to be sufficiently smaller than the scale of the total-energy differences we discuss in Sec. S.V to not alter any of our conclusions.

When attempting to approximate the localized atomic-like 4f shell with the Kohn–Sham DFT, one faces a severe issue that the many-body wave function of the 4f shell is typically far from a single-determinant form, whereas the Kohn–Sham state is a single determinant by definition. Fortunately, Eu is an exception to this rule.

In the ferromagnetic phase of EuS, the $4f^7$ shell has zero orbital moment and its spin 7/2 points along the quantization axis. This state is very well approximated by a single determinant

$$|\Psi_\uparrow\rangle = \prod_{m=-3}^{3} \hat{f}^\dagger_{m\uparrow}|0\rangle\,. \qquad \text{(S2)}$$

To demonstrate that, we compare this state with the ground state of our LDA+DMFT impurity model. To make the exposition more transparent, we reduce this model to just the 4f shell containing the Coulomb repulsion and the spin-orbit coupling $\zeta(\mathbf{l}\cdot\mathbf{s})$, with $\zeta = 183$ meV as found in the LDA+DMFT calculations. The ground

TABLE S.I. Summary of open-core approximations to the states of the 4f shell utilized in this study. The non-magnetic state $|^7F_0\rangle$ is approximated by a spin-polarized state since it provides a much better total energy than the corresponding spin-restricted state (see text for details).

| state | open-core approximation | | | |
|---|---|---|---|---|
| | $n_{4f}^{5/2\uparrow}$ | $n_{4f}^{7/2\uparrow}$ | $n_{4f}^{5/2\downarrow}$ | $n_{4f}^{7/2\downarrow}$ |
| $4f^7$ $\|^8S_{7/2}, m = 7/2\rangle$ | 3.00 | 4.00 | 0.00 | 0.00 |
| $4f^6$ $\|^7F_6, m = 6\rangle$ | 2.14 | 3.86 | 0.00 | 0.00 |
| $4f^6$ $\|^7F_0\rangle$ | 3.00 | 3.00 | 0.00 | 0.00 |
| spin-restricted $4f^7$ | 3.00 | 0.50 | 3.00 | 0.50 |
| spin-restricted $4f^6$ | 3.00 | 0.00 | 3.00 | 0.00 |

state of the 4f shell is

$$\left|^8S_{7/2}, m = 7/2\right\rangle = 0.987|\Psi_\uparrow\rangle - \sum_{m=-3}^{2} a_m \hat{f}^\dagger_{m+1\downarrow}\hat{f}_{m\uparrow}|\Psi_\uparrow\rangle + \dots \quad \text{(S3)}$$

with the amplitudes of the largest additional terms $a_m = \{0.048, 0.064, 0.073, 0.076, 0.072, 0.058\}$. The mixing of the minority-spin electrons due to spin-orbit coupling is only tiny, the exchange splitting of the 4f shell is the dominant effect. In the open-core approximation, we thus fill all majority-spin 4f states and keep all minority-spin states empty (Table S.I).

To estimate how the valence electronic structure looks in the paramagnetic phase, that is, in a state without the exchange field induced by the polarized 4f electrons, we calculate also a non-magnetic (spin-restricted) solution with equal occupation of $\uparrow$ and $\downarrow$ states. The state of the 4f shell is defined by occupations $n_{4f}^{5/2} = 6$ and $n_{4f}^{7/2} = 1$. Note that this state is very different from the fluctuating local-moment state in the paramagnetic phase of EuS. This means that although the non-4f bands from the spin-restricted calculations provide a reasonable approximation to the non-4f bands in the paramagnet, the spin-restricted total energy is very far from the total energy of the paramagnetic phase.

The band structures of the non-magnetic and ferromagnetic states found in the open-core approximation are shown in Fig. S1. The gap between S 3p and Eu 5d bands, underestimated in LDA, was increased by applying an extra potential $-2.0$ eV acting on the S 3p states. A larger value than the $-1.5$ eV shift applied in the tight-binding model in Sec. S.III is needed since the extra potential acts only in the sulfur muffin-tin sphere and not on the entire S 3p Wannier function.

Figure S1 illustrates that the two computational methods used in this study (LDA+DMFT and open-core approximation) provide very similar predictions for the non-4f bands. It also points to some limitations of the two methods: the already mentioned missing exchange splitting of the Eu 5d bands in our implementation of LDA+DMFT (this exchange splitting is present in the open-core method), and an underestimated exchange splitting of the S 3p bands in the open-core approximation, which is due to the hybridization between S 3p and Eu 4f states being completely removed in this method (this hybridization is present in the LDA+DMFT method).

## S.V. LOCALIZED EXCITON IN A SUPERCELL

The localized exciton formed by a hole in the 4f shell of an Eu atom and a valence charge attracted to this hole is modeled in a (large) supercell where the 4f shell of one of the Eu atoms is constrained to have six instead of seven electrons. The calculations utilize the open-core method, which offers a straightforward way of implementing this constraint.

The exciton with the smallest excitation energy is most likely formed by the ground-state of $4f^6$ and the screening valence electron. This $4f^6$ ground state, the singlet $^7F_0$, is essentially impossible to model in DFT due to its multi-reference nature. In the ionic model used in Sec. S.IV it has the form

$$\left|^7F_0\right\rangle = 0.362\Big(|X_\uparrow\rangle + |X_\downarrow\rangle\Big) - 0.227\Big(\hat{f}^\dagger_{3\downarrow}\hat{f}_{2\uparrow}|X_\uparrow\rangle + \hat{f}^\dagger_{-3\uparrow}\hat{f}_{-2\downarrow}|X_\downarrow\rangle\Big) + \dots, \quad \text{(S4)}$$

where we introduced determinants

$$|X_\uparrow\rangle = \prod_{m=-3}^{2} \hat{f}^\dagger_{m\uparrow}|0\rangle \quad \text{and} \quad |X_\downarrow\rangle = \prod_{m=-2}^{3} \hat{f}^\dagger_{m\downarrow}|0\rangle \quad \text{(S5)}$$

that have their total spin and total orbital moments antiparallel.

A state that can be accurately modeled by DFT must be maximally polarized similarly to the $4f^7$ ground state $^8S_{7/2}$, Eq. (S3). In the series $^7F_0, {^7F_1}, {^7F_2}, \dots, {^7F_6}$, arising from splitting of the $L = 3$, $S = 3$ $4f^6$ manifold by the spin-orbit coupling, such maximally polarized state is $^7F_6$, namely

$$\left|^7F_6, m = 6\right\rangle = 0.978|\Phi_\uparrow\rangle - \sum_{m=-2}^{2} b_m \hat{f}^\dagger_{m+1\downarrow}\hat{f}_{m\uparrow}|\Phi_\uparrow\rangle + \dots, \quad \text{(S6)}$$

where the leading determinant is (the total spin parallel to the total orbital moment)

$$|\Phi_\uparrow\rangle = \prod_{m=-2}^{3} \hat{f}^\dagger_{m\uparrow}|0\rangle \quad \text{(S7)}$$

and where the amplitudes of the larges additional spin-mixing terms are $b_m = \{0.074, 0.085, 0.096, 0.101, 0.096\}$. The determinant $|\Phi_\uparrow\rangle$ corresponds to occupations $n_{4f}^{5/2\uparrow} =$

TABLE S.II. Excitation energy $\Delta$ and the excess of the valence electrons at the site with the 4f hole $\Delta n_{\mathrm{val}}$ calculated in different supercells in the ferromagnetic (FM) or non-magnetic (NM) state, and for spin-polarized (SP) or non-magnetic $4f^6$ shell at the excited atom. The excess $\Delta n_{\mathrm{val}}$ is counted in the atomic sphere with radius $3.1\,a_{\mathrm{B}}$. The model with the best total energies is shown in red.

| supercell | number of atoms | host | $4f^6$ | $\Delta$ (eV) | $\Delta n_{\mathrm{val}}$ |
|---|---|---|---|---|---|
| $2\times2\times2$ | 64 | FM | SP | 2.1 | 0.56 |
| $3\times3\times3$ | 216 | FM | SP | 2.2 | 0.54 |
| $4\times4\times4$ | 512 | FM | SP | 2.4 | 0.54 |
| $2\times2\times2$ | 64 | FM | NM | 6.5 | 0.55 |
| $3\times3\times3$ | 216 | FM | NM | 6.6 | 0.54 |
| $4\times4\times4$ | 512 | FM | NM | 6.8 | 0.54 |
| $2\times2\times2$ | 64 | NM | NM | 0.7 | 0.52 |
| $3\times3\times3$ | 216 | NM | NM | 0.8 | 0.51 |
| $4\times4\times4$ | 512 | NM | NM | 1.1 | 0.51 |

2.14 and $n_{4f}^{7/2\uparrow} = 3.86$. In Wien2k, these occupations give total energy approximately 0.6 eV higher than occupations $n_{4f}^{5/2\uparrow} = 3$ and $n_{4f}^{7/2\uparrow} = 3$ that correspond to the determinant $|X_\uparrow\rangle$, Eq. (S5), which is one of the leading components of the $4f^6$ ground state ${}^7F_0$, Eq. (S4). In the same time, the state ${}^7F_6$ is approximately 0.7 eV above the ground state ${}^7F_0$ in our LDA+DMFT solution (manifested as the width of the occupied 4f bands in Fig. S1). The occupations $n_{4f}^{5/2\uparrow} = 3$ and $n_{4f}^{7/2\uparrow} = 3$ therefore provide a good estimate for the ground-state energy of the $4f^6$ shell. We employ these occupations in the following when we refer to the spin-polarized $4f^6$ state.

Table S.II summarizes the basic characteristics of the excitons computed in supercells of increasing size (we use integer multiples of the conventional 8-atom cell). We list the excitation energy $\Delta = E_{\mathrm{exc}} - E_{\mathrm{clean}}$ defined as a difference between the total energy of a supercell with an exciton and the total energy of a supercell without any excitons, as well as the excess of the valence electrons $\Delta n_{\mathrm{val}}$ at the excited Eu site. The Eu 5d densities of states at the excited atom are plotted in Fig. S3. Unlike Secs. S.III and S.IV we did not add any extra potential to the S 3p states to keep the LDA total-energy functional unmodified. Both Table S.II and Fig. S3 show that the convergence with respect to the supercell size is rather slow and that even the 512-atom supercell may not provide entirely converged data. At present, however, we could not afford to work with larger supercells. Already now we use a slightly smaller plane-wave cutoff than in Secs. S.III and S.IV, namely $R_{\mathrm{MT}}(\mathrm{S}) \times K_{\mathrm{max}} = 7.5$. The k-point mesh is kept at least as dense as in the primitive-cell calculations, we employ meshes $10\times10\times10$, $5\times5\times5$ and $5\times5\times5$ for supercells $2\times2\times2$, $3\times3\times3$ and $4\times4\times4$, respectively. All calculations again use the experimental lattice constant and no geometry optimization is performed.

Besides the cases with the spin-polarized $4f^7$ and $4f^6$ shells, which provide the best approximation for the to-

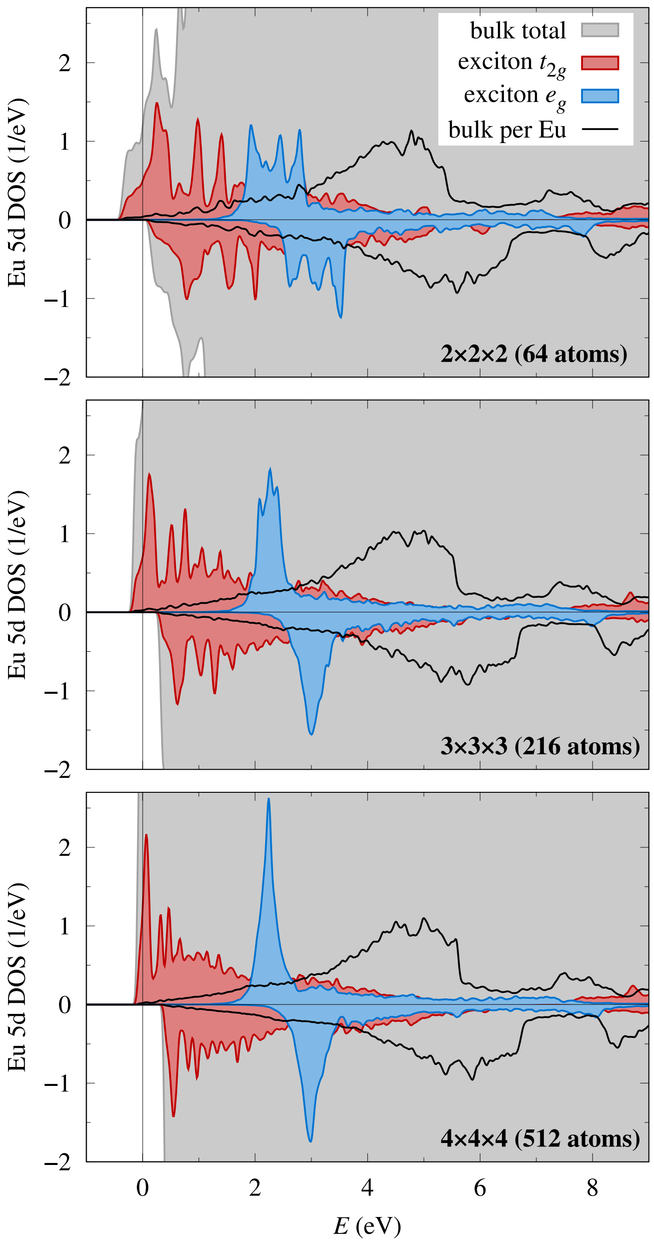


FIG. S3. The unoccupied Eu 5d density of states at the excited atom computed in supercells of increasing size (from top to bottom). The ferromagnetic solutions are shown, positive values correspond to majority-spin states, negative values to minority-spin states. Even the $3\times3\times3$ supercell (middle) is apparently too small as the DOS features continue to narrow all the way to the largest supercell studied.

tal energy, Table S.II lists also calculations with spin-restricted $4f^6$ shell at the excited atom ($n_{4f}^{5/2} = 6$ and $n_{4f}^{7/2} = 0$) embedded in the spin-polarized bulk as well as in the spin-restricted bulk. These calculations indicate that the spin-restricted $4f^6$ shell has about 4.4 eV higher energy than the spin-polarized $4f^6$ shell and hence it is not a good model for the non-magnetic ${}^7F_0$ state. The completely spin-restricted calculations that we use

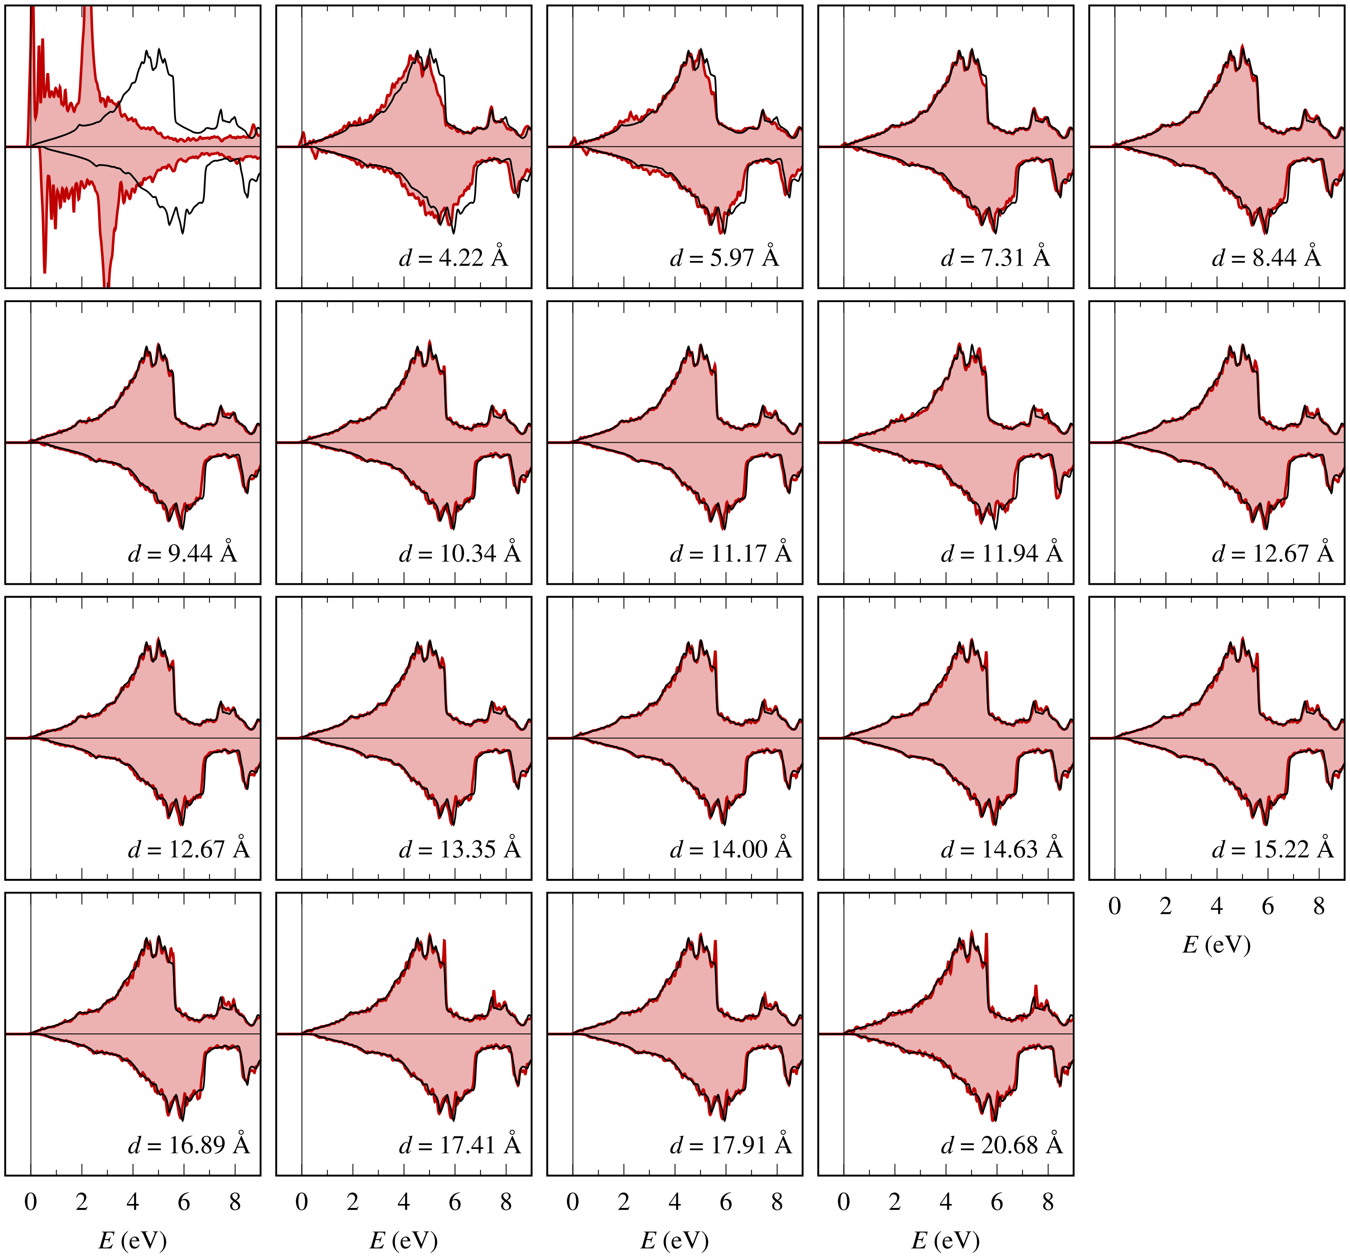


FIG. S4. The local Eu 5d density of states (red) at all nonequivalent Eu sites in the $4 \times 4 \times 4$ supercell ordered by their increasing distance $d$ from the site with the 4f hole (top left panel). The bulk DOS per Eu atom is shown in black. The exciton is indeed localized, the deviations of the local DOS from the bulk DOS are only small outside of the excited site.

to approximate the density of states in the paramagnetic phase (Fig. 4) are apparently not very useful for any total-energy considerations since they provide excitation energy $\Delta$ that is quite far from the excitation energy $\approx 2.5$ eV determined from RIXS and optical absorption spectroscopy.

Finally, we illustrate that the computed exciton is a local object confined to the vicinity of the Eu atom with the 4f hole. To do so, we plot the local Eu 5d density of states at each of the Eu sites in the supercell with increasing distance from the excited atom (Fig. S4). Only the excited atom displays substantial modifications of the local 5d DOS, other sites show just tiny differences from the bulk DOS that are discernible only at the three or four nearest Eu neighbors.

## S.VI. INTENSITY OF QUADRUPOLAR EMISSION

We estimate the intensity of quadrupolar transitions relative to the dipolar transitions on the basis of exper-

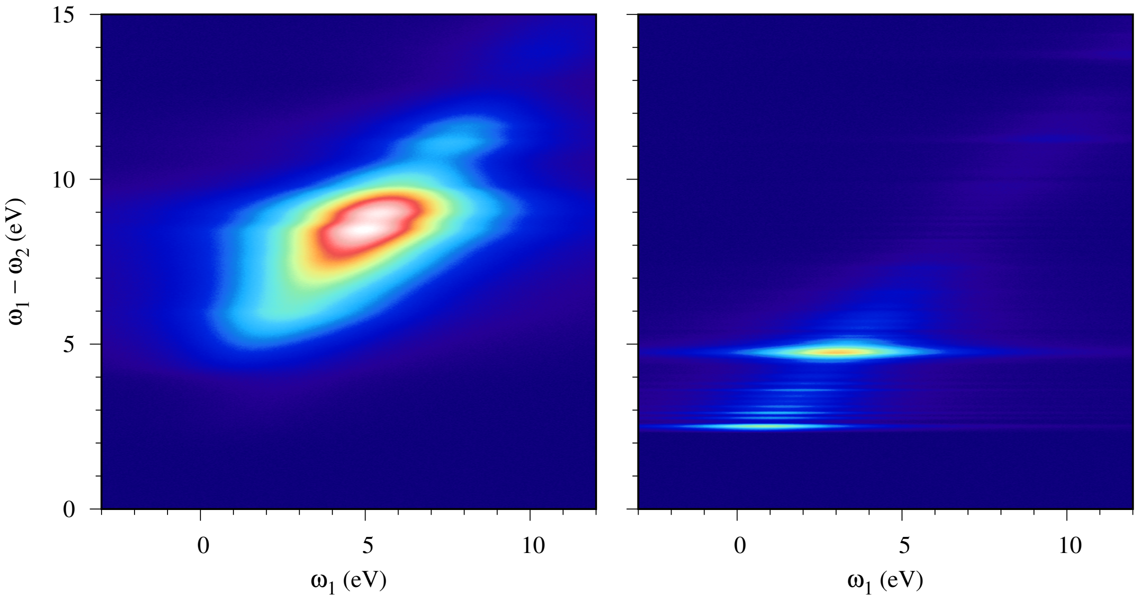


FIG. S5. The dipole (left) and quadrupole (right) components of the RIXS computed from Eqs. (1) and (2), respectively. They are combined to one figure shown as Fig. 2a in the main text.

imental data reported in [S19], where the quadrupolar pre-edge structure was investigated at the $L_3$ absorption edge in a series of rare-earth intermetallics $R_2Fe_{14}B$. The ratio of the pre-edge intensity $E_2$ (absorption to the 4f states) to the main dipolar intensity $E_1$ (absorption to the 5d states) was found to be approximately

$$\frac{E_2}{E_1} \approx 7.5 \times 10^{-7} Z^2 (14 - n_f)\,, \tag{S8}$$

where $Z$ is the atomic number of the rare-earth atom and $n_f$ is the number of 4f electrons (see the fit shown in Fig. 7 of [S19]). If we write each intensity as a product of a transition probability per a single-particle final state and the number of available final states, $E_1 = p_D(10 - n_d)$ and $E_2 = p_Q(14 - n_f)$, we get

$$\frac{p_Q}{p_D} = 7.5 \times 10^{-7} Z^2 (10 - n_d) \tag{S9}$$

for the ratio of quarupolar and dipolar transition probabilities. Assuming that $n_d$ is practically constant across the $R_2Fe_{14}B$ series and equal to approximately two, as found computationally for $Nd_2Fe_{14}B$ in [S20], we arrive at an estimate

$$\frac{p_Q}{p_D} = 0.024 \tag{S10}$$

for Eu. Although this result is deduced for absorption, we assume that the ratio of the emission processes will be similar and we use this $p_Q/p_D$ value when combining RIXS maps from dipolar and quadrupolar emission channels computed from Eqs. (1) and (2) of the main text. The combined RIXS map is shown in Fig. 2a. For completeness, we present also the individual components (dipole and quadrupole emission channels) in Fig. S5.

## S.VII. INDIRECT RIXS PROCESSES

All the discussion in the present paper is about *direct* RIXS processes, in which the excited electron-hole pair in the final state results directly from the absorption and emission of the incoming and outgoing photon. There exist also *indirect* RIXS excitations that are due to the core-hole potential perturbing the valence electronic structure in the intermediate state of the RIXS process and that can be seen as shake-up excitations [S21, S22]. They can appear in addition to the electron-hole pairs from the direct RIXS, or separately when they emerge in the processes that produce the elastic peak ($\omega_2 = \omega_1$). The indirect RIXS could reach excitations of the $4f^7$ configuration (but the first is $^6P_{7/2}$ at roughly 4 eV [S23], which does not coincide with any of the observed RIXS features) or it could provide and alternative (dipole-allowed) way to excite the $4f^6 5d^1$ excitons. The indirect RIXS can be estimated in the DFT+DMFT impurity model by methods analogous to [S24–S26] if we neglect the modification of the local 5d density of states due to the Coulomb interaction with the 4f hole, which, given our other results, looks like a rather crude approximation. When we tested this approach, we found that the intensity of the indirectly excited $4f^7$ and $4f^6 5d^1$ features is very weak when compared to the direct signal given by Eq. (1). Without the 4f–5d Coulomb interaction, these indirect excitations would show a strong dependence on the scattering angle [S24], which could be a way to distinguish them from excitations seen in the quadrupole emission channel discussed in the present paper. We did not explore this possibility as it would require performing additional experiments as well as generalizing the impurity model to include the modification of the local 5d DOS due to the 4f hole.

* lucia.amidani@esrf.fr
† kolorenc@fzu.cz

[S1] P. Glatzel, A. Harris, P. Marion, M. Sikora, T.-C. Weng, C. Guilloud, S. Lafuerza, M. Rovezzi, B. Detlefs, and L. Ducotté, The five-analyzer point-to-point scanning crystal spectrometer at ESRF ID26, J. Synchrotron. Rad. **28**, 362 (2021).
[S2] A. V. Fedorov, G. Poelchen, S. V. Eremeev, S. Schulz, A. Generalov, C. Polley, C. Laubschat, K. Kliemt, N. Kaya, C. Krellner, E. V. Chulkov, K. Kummer, D. Yu. Usachov, A. Ernst, and D. V. Vyalikh, Insight into the temperature evolution of electronic structure and mechanism of exchange interaction in EuS, J. Phys. Chem. Lett. **12**, 8328 (2021).
[S3] J. Kolorenč, A. B. Shick, and A. I. Lichtenstein, Electronic structure and core-level spectra of light actinide dioxides in the dynamical mean-field theory, Phys. Rev. B **92**, 085125 (2015), arxiv:1504.07979 [cond-mat.str-el].
[S4] B. Chatterjee and J. Kolorenč, Electronic structure and magnetism in $UGa_2$: DFT+DMFT approach, Phys. Rev. B **103**, 205146 (2021), arxiv:2102.08224 [cond-mat.str-el].
[S5] P. Blaha, K. Schwarz, F. Tran, R. Laskowski, G. K. H. Madsen, and L. D. Marks, WIEN2k: An APW+lo program for calculating the properties of solids, J. Chem. Phys. **152**, 074101 (2020).
[S6] P. Wachter, The optical electrical and magnetic properties of the europium chalcogenides and the rare earth pnictides, Crit. Rev. Solid State Sci. **3**, 189 (1972).
[S7] I. Souza, N. Marzari, and D. Vanderbilt, Maximally localized Wannier functions for entangled energy bands, Phys. Rev. B **65**, 035109 (2001), arxiv:cond-mat/0108084.
[S8] A. A. Mostofi, J. R. Yates, Y.-S. Lee, I. Souza, D. Vanderbilt, and N. Marzari, Wannier90: A tool for obtaining maximally-localised Wannier functions, Comput. Phys. Commun. **178**, 685 (2008), arxiv:0708.0650 [cond-mat.mtrl-sci].
[S9] J. M. An, S. V. Barabash, V. Ozolins, M. van Schilfgaarde, and K. D. Belashchenko, First-principles study of phase stability of Gd-doped EuO and EuS, Phys. Rev. B **83**, 064105 (2011), arxiv:1012.4026 [cond-mat.str-el].
[S10] M. Schlipf, M. Betzinger, M. Ležaić, C. Friedrich, and S. Blügel, Structural, electronic, and magnetic properties of the europium chalcogenides: A hybrid-functional DFT study, Phys. Rev. B **88**, 094433 (2013).
[S11] I. L. M. Locht, Y. O. Kvashnin, D. C. M. Rodrigues, M. Pereiro, A. Bergman, L. Bergqvist, A. I. Lichtenstein, M. I. Katsnelson, A. Delin, A. B. Klautau, B. Johansson, I. Di Marco, and O. Eriksson, Standard model of the rare earths analyzed from the Hubbard I approximation, Phys. Rev. B **94**, 085137 (2016), arxiv:1512.02848 [cond-mat.str-el].
[S12] R. D. Cowan, *The Theory of Atomic Structure and Spectra* (University of California Press, Berkeley, 1981).
[S13] H. Ogasawara, A. Kotani, and B. T. Thole, Lifetime effect on the multiplet structure of 4d x-ray-photoemission spectra in heavy rare-earth elements, Phys. Rev. B **50**, 12332 (1994).
[S14] P. Cotti and P. Munz, Photoemissionsmessungen an Europiumchalkogeniden, Phys. cond. matter **17**, 307 (1974).
[S15] S. K. Malik, F. J. Arlinghaus, and W. E. Wallace, Spin-polarized energy-band structure of $YCo_5$, $SmCo_5$, and $GdCo_5$, Phys. Rev. B **16**, 1242 (1977).
[S16] M. S. S. Brooks, L. Nordström, and B. Johansson, 3d-5d band magnetism in rare earth-transition metal intermetallics: Total and partial magnetic moments of the $RFe_2$ (R=Gd-Yb) Laves phase compounds, J. Phys.: Condens. Matter **3**, 2357 (1991).
[S17] WIEN2k-FAQ: "open core" treatment of 4(5)f electrons (2001).
[S18] G. Y. Guo, H. Ebert, W. M. Temmerman, K. Schwarz, and P. Blaha, Relativistic effects on the structural and magnetic properties of iron, Solid State Commun. **79**, 121 (1991).
[S19] F. Bartolomé, M. H. Krisch, D. Raoux, and J.-M. Tonnerre, Quadrupolar excitation channels at the $L_3$ edge of rare-earth ions probed by resonant inelastic x-ray scattering, Phys. Rev. B **60**, 13497 (1999).
[S20] L. Nordström, B. Johansson, and M. S. S. Brooks, Calculation of the electronic structure and the magnetic moments of $Nd_2Fe_{14}B$, J. Phys.: Condens. Matter **5**, 7859 (1993).
[S21] J. van den Brink and M. van Veenendaal, Correlation functions measured by indirect resonant inelastic X-ray scattering, EPL **73**, 121 (2006).
[S22] M. van Veenendaal, *Theory of Inelastic Scattering and Absorption of X-rays* (Cambridge University Press, Cambridge, UK, 2015).
[S23] J. J. Joos, D. Poelman, and P. F. Smet, Energy level modeling of lanthanide materials: Review and uncertainty analysis, Phys. Chem. Chem. Phys. **17**, 19058 (2015).
[S24] A. Kotani, K. O. Kvashnina, S. M. Butorin, and P. Glatzel, Spectator and participator processes in the resonant photon-in and photon-out spectra at the Ce $L_3$ edge of $CeO_2$, Eur. Phys. J. B **85**, 257 (2012).
[S25] J. Kolorenč, Theory of resonant x-ray emission spectra in compounds with localized f electrons, Physica B **536**, 695 (2018), arxiv:1707.03158 [cond-mat.str-el].
[S26] A. Hariki, M. Winder, T. Uozumi, and J. Kuneš, LDA+DMFT approach to resonant inelastic x-ray scattering in correlated materials, Phys. Rev. B **101**, 115130 (2020), arxiv:1911.10366 [cond-mat.str.el].
